# Supplementary material for: Enhanced Anomalous Hall Effect in Magnetic Topological Semimetal Co$_3$Sn$_{2-x}$In$_x$S$_2$
Source: arXiv:2003.02412 source file (2020-03-05)
Supplement: Supplementary file 1 [file CSIS_AHE_SI_Mar1.pdf]

# Supplementary Information
# Enhanced Anomalous Hall Effect in Magnetic Topological Semimetal $Co_3Sn_{2-x}In_xS_2$


Huibin Zhou,[1] Guoqing Chang,[2] Guangqiang Wang,[1] Xin Gui,[3] Xitong Xu,[1] Jia-Xin Yin,[2] Zurab Guguchia,[2,4] Songtian S. Zhang,[2] Tay-Rong Chang,[5] Hsin Lin,[6] Weiwei Xie,[3] M. Zahid Hasan,[2,7,8] and Shuang Jia[1,9,10,11,*]

[1] *International Center for Quantum Materials, School of Physics, Peking University, China*

[2] *Laboratory for Topological Quantum Matter and Advanced Spectroscopy(B7), Department of Physics, Princeton University, Princeton, NJ 08544, USA*

[3] *Department of Chemistry, Louisiana State University, Baton Rouge, LA 70803, USA*

[4] *Laboratory for Muon Spin Spectroscopy, Paul Scherrer Institute, CH-5232 Villigen PSI, Switzerland*

[5] *Department of Physics, National Cheng Kung University, Tainan 701, Taiwan*

[6] *Institute of Physics, Academia Sinica, Taipei 11529, Taiwan*

[7] *Princeton Institute for Science and Technology of Materials, Princeton University, Princeton, NJ 08544, USA*

[8] *Materials Science Division, Lawrence Berkeley National Laboratory, Berkeley, CA 94720, USA*

[9] *Collaborative Innovation Center of Quantum Matter, Beijing 100871, China*

[10] *CAS Center for Excellence in Topological Quantum Computation, University of Chinese Academy of Sciences, Beijing 100190, China*

[11] *Beijing Academy of Quantum Information Sciences, West Building 3, No. 10 Xibeiwang East Road, Haidian District, Beijing 100193, China*

* gwljiashuang@pku.edu.cn

## I. METHOD

All $Co_3Sn_{2-x}In_xS_2$ crystals used in the present study were grown by the Bridgeman technique [1]. Five grams raw materials of Co and S pieces and Sn and In ingots were mixed together with the stoichiometric molar ratio of Co : S : Sn : In = 3 : 2 : $2-x$ : $x$ and then placed in a dry alumina crucible, which was sealed in a fused silica ampoule under argon environment. The ampoule was then placed in a furnace and heated to 1000 °C over 4 h and kept for 24 h, then slowly cooled to 800 °C at a rate of 3 °C/h. After the steps above, the yielded crystals have typical length of 2 cm and diameter of 1 cm.

The crystal structure of $Co_3Sn_{2-x}In_xS_2$ was examined by powder X-ray diffraction(PXRD) measurements using a Rigaku Mini-flux 600 diffractometer with Cu $K_\alpha$ radiation. Single crystals and orientations were assigned by Laue X-ray diffraction. The composition was determined by energy dispersive X-ray spectroscopy (EDS) in a Helios NanoLab$^{TM}$ 600i DualBeam System. The lattice constants were refined from the PXRD data by the Rietveld method using Rietica software. The obtained lattice parameters $a$ and $c$ show linear dependence on $x$ (Fig. 1 in main text).

Longitudinal and Hall resistivity measurements were performed in a commercial system (PPMS, Quantum Design) by standard four-probe method with silver paste contacts cured at room temperature. Magnetization as a function of temperature with a range of 2∼200 K was measured in a Quantum Design MPMS superconducting quantum interference device(SQUID) magnetometer under magnetic field of 0.5 T applied parallel to the easy $c$ axis.

## II. ANOMALOUS HALL CONDUCTIVITY IN MASSIVE DIRAC MODEL

In the massive Dirac model, the intrinsic anomalous Hall conductivity(AHC) is captured by

$$\sigma_{xy}^{int} = \begin{cases} -\frac{e^2}{2h} \cdot \frac{\Delta}{\varepsilon_F}, & \text{if } \varepsilon_F < -\Delta \\ \frac{e^2}{2h}, & \text{if } -\Delta < \varepsilon_F < \Delta \\ \frac{e^2}{2h} \cdot \frac{\Delta}{\varepsilon_F}, & \text{if } \varepsilon_F > \Delta \end{cases} \quad (1)$$

where $\varepsilon_F$ is the Fermi level and $2\Delta$ is the size of the Dirac gap [2]. Because the massive Dirac fermions at the K and K′ in the kagomé lattice contribute similarly to Berry curvature,

the value of the intrisic AHC from Eq. (1) is doubled. We plot the energy dependence of intrinsic AHC in Fig. S1. It can be seen that the AHC remains constant in the Dirac gap but drops with a tail outside the gap.

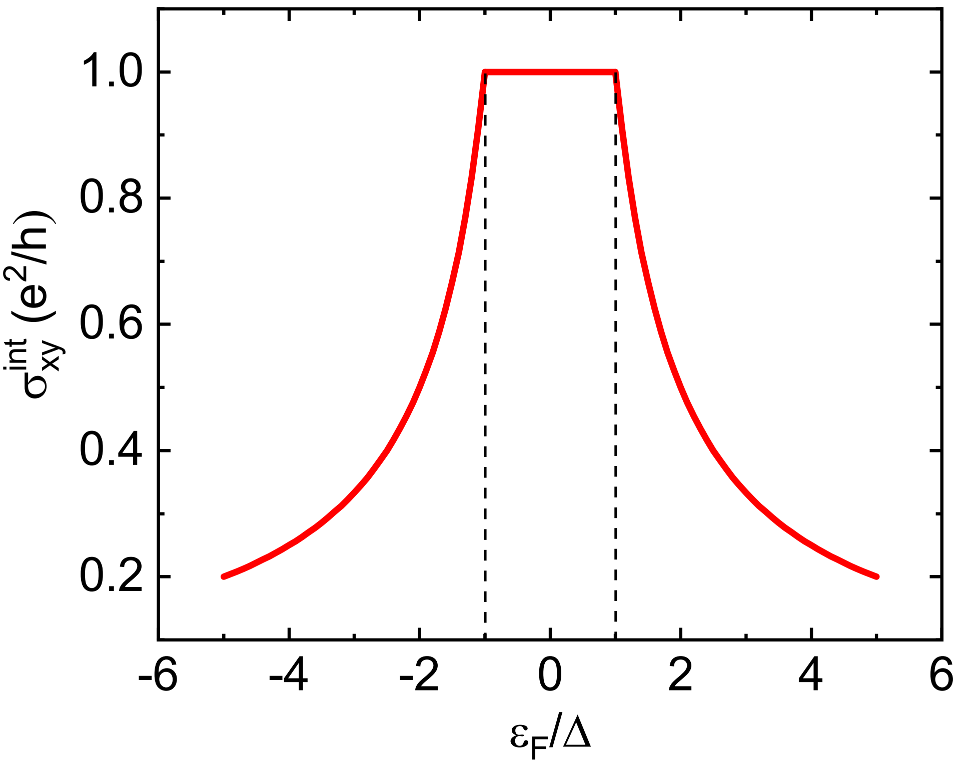


FIG. S1: The intrinsic anomalous Hall conductivity as a function of the Fermi energy $\varepsilon_F$ in the units of $e^2/h$, $\Delta$ represents half of the band gap.

## III. SCALING OF ANOMALOUS HALL CONDUCTIVITY

Figure S2 shows the anomalous Hall conductivity $\sigma_{\rm xy}^{\rm A}$ as a function of longitudinal conductivity $\sigma_{\rm xx}$ for different samples in $Co_3Sn_{2-x}In_xS_2$. The two black lines are $\sigma_{\rm xy}^{\rm A} \propto \sigma_{xx}^{1.6}$ for dirty regime and $\sigma_{\rm xy}^{\rm A} = \text{const}$ for intermediate regime, respectively. The anomalous Hall effect (AHE) in $Co_3Sn_{2-x}In_xS_2$ is approximately located in the crossover from the intermediate ($10^4 - 10^6$ S/cm) to the dirty ($\sigma_{\rm xx} < 10^4$ S/cm) region [3].

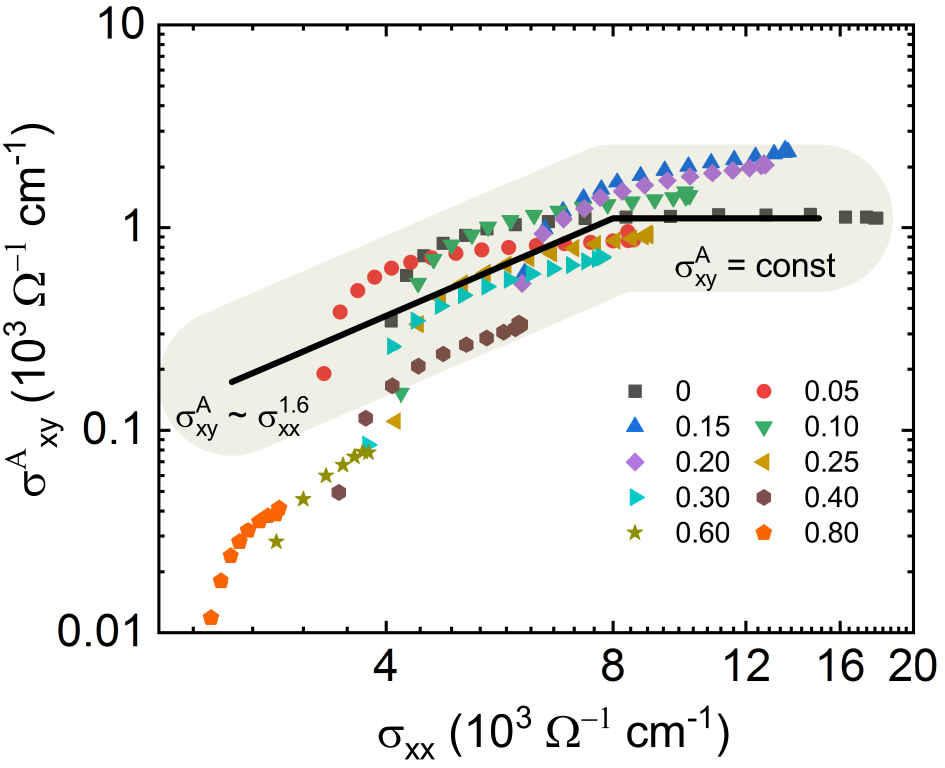


FIG. S2: Anomalous Hall conductivity $\sigma^A_{xy}$ as a function of longitudinal conductivity $\sigma_{xx}$ for different samples in $Co_3Sn_{2-x}In_xS_2$.

## IV. DETERMINATION OF FERMI ENERGY

We use the following equation to estimate the Fermi energy $E_F$ of indium-substituted samples in accordance to the rigid band of $Co_3Sn_2S_2$:

$$N = \int_0^{E_F} N(E)dE \tag{2}$$

Where $N(E)$ is the density of state per unit volume, $N$ is the carrier concentration and $E_F$ is the Fermi energy for $Co_3Sn_{2-x}In_xS_2$. The indium substitution removes one electron for sustituting each tin atom. Figure S3 shows the inferred $E_F$ for $Co_3Sn_{2-x}In_xS_2$.

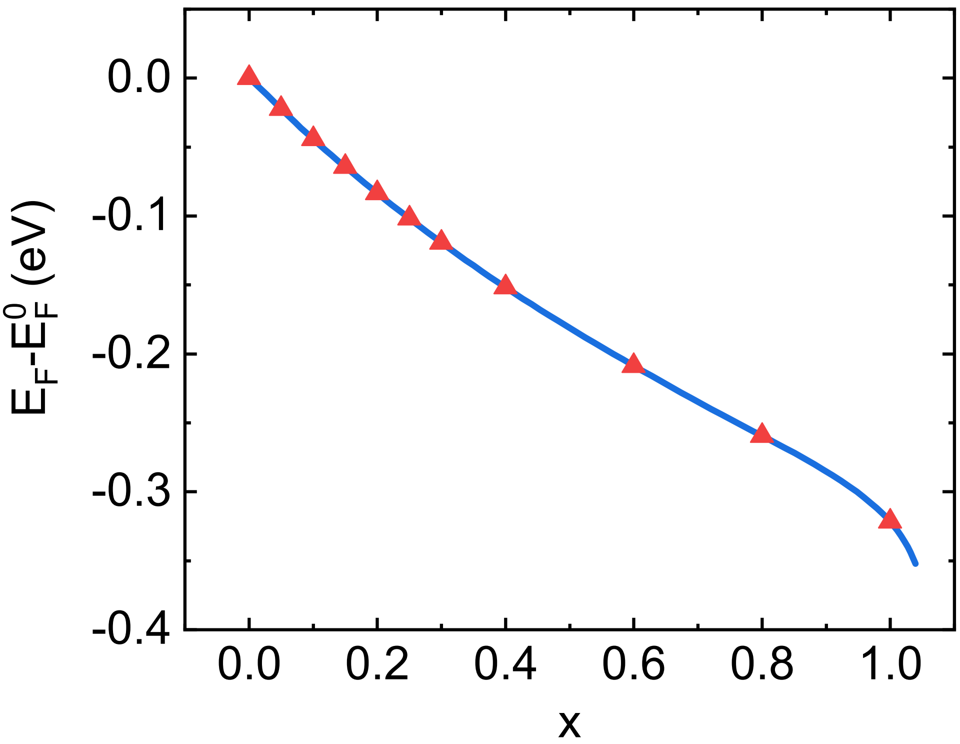


FIG. S3: The shift of Fermi energy with increasing In content $x$ for $Co_3Sn_{2-x}In_xS_2$. The red dots represent the indium concentration for the samples in this study.

## V. MOBILITY AND SKEW SCATTERING AHE

Figure S4 shows the hole mobility for $x \leq 0.6$. The mobility of pristine $Co_3Sn_2S_2$ ($5 \times 10^2$ cm$^2$V$^{-1}$s$^{-1}$, not shown here) from two-band model is much larger than the doped samples. For $0.05 \leq x \leq 0.15$, the mobility is near 80 cm$^2$V$^{-1}$s$^{-1}$ and then gradually drops with increasing $x$ when $x > 0.15$. We notice that when $x > 0.15$, the skew-scattering-bearing AHC ($\sigma_{xy}^{sk}$) is linearly dependent on the mobility (Fig. S5). For $x < 0.15$, the $\sigma_{xy}^{sk}$ apparently deviates from the linear relation. These differences can be understood in the rigid band model, in which the skew scattering AHE should change significantly when the Fermi level crosses the SOC gap from x<0.15 to >0.15.

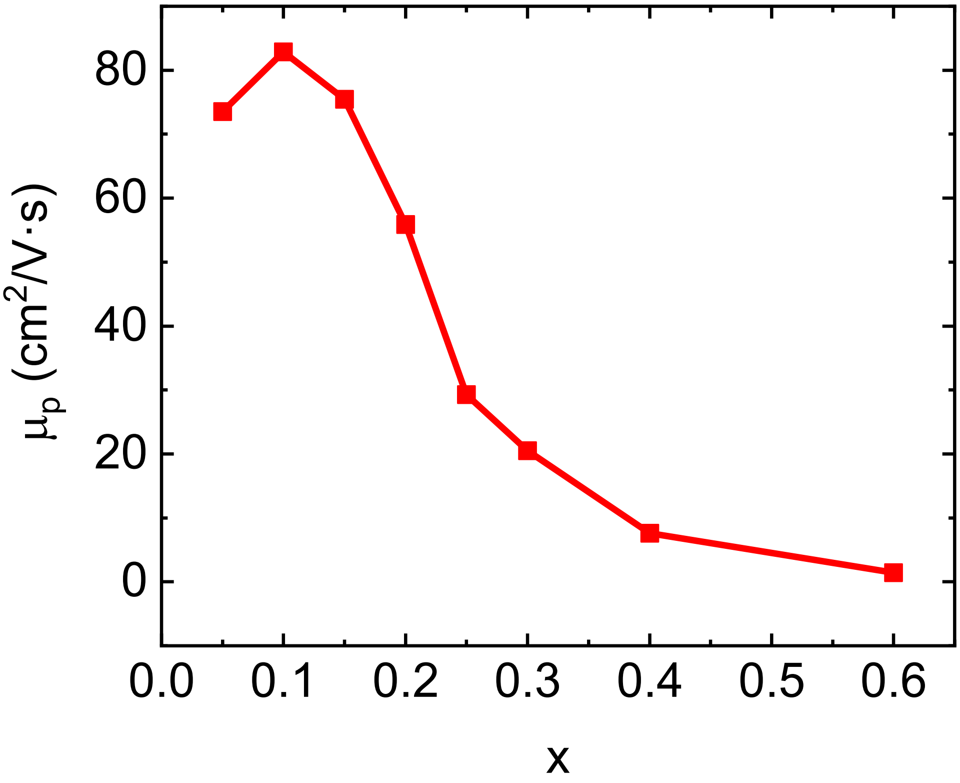


FIG. S4: The doping dependence of hole mobility.

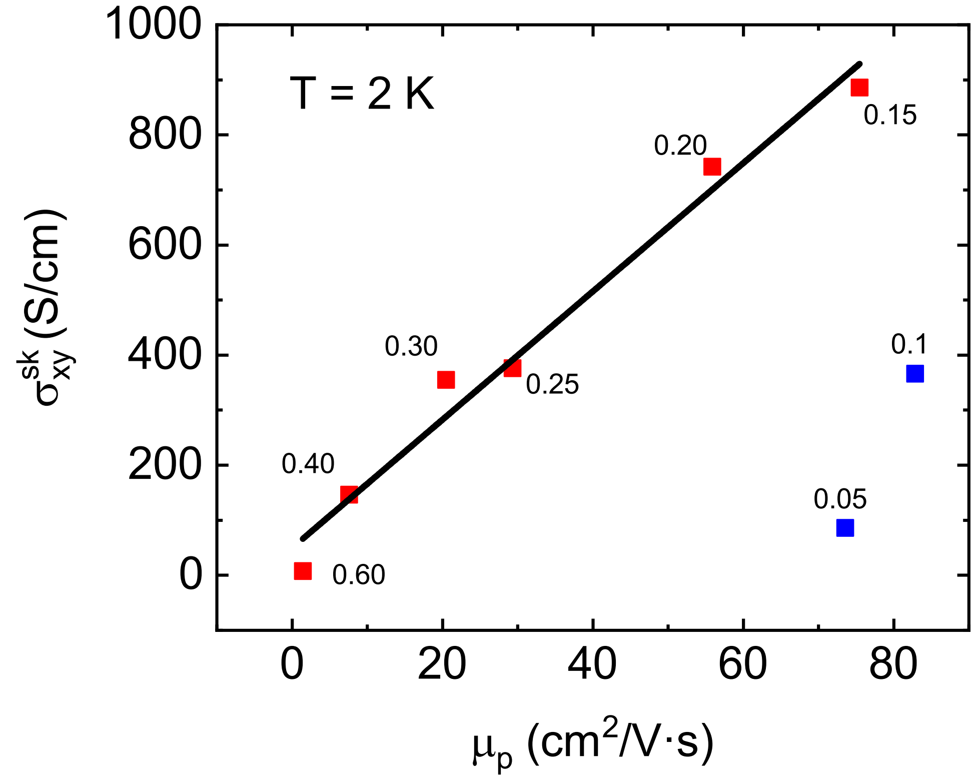


FIG. S5: The AHC of skew scattering vs mobility

[1] M. Holder, Y. S. Dedkov, A. Kade, and Rosner, Phys. Rev. B **79**, 205116 (2009).

[2] N. A. Sinitsyn, A. H. MacDonald, T. Jungwirth, V. K. Dugaev, and J. Sinova, Phys. Rev. B **75**, 045315 (2007).

[3] T. Miyasato, N. Abe, T. Fujii, A. Asamitsu, S. Onoda, Y. Onose, N. Nagaosa, and Y. Tokura, Phys. Rev. Lett. **99**, 086602 (2007).
